# Supplementary material for: CANOE: Classically Assisted Non-Orthogonal Eigensolver
Source: arXiv:2603.13188 source file (2026-03-13)
Supplement: Supplementary file 1 [file appendix_D_plateau_behavior.tex]

% Appendix D moved out of the main manuscript.
\section{Unresolved-overlap weight as a diagnostic of plateau behavior}
\label{appendix:plateau_sampled_results}

To interpret the plateau behavior in the histogram-based error
convergence curves, especially panel (d) of
\cref{fig:overlap_benchmark}, it is difficult to rely on a single
scalar quantity. We tested several diagnostics, and among them the
quantity that showed the clearest empirical correlation with the
plateau was the unresolved-overlap weight
$W_{\mathrm{unres}}$. The purpose of this quantity is to estimate how
much of the exact ground-state vector lies in overlap directions that
are not resolved at a given sampling noise level.

Let $\ell$ denote a molecule, $s$ a shot count, and $k$ a seed or run
index. For each sampled run we estimate a resolution threshold
$\tau_{\ell,s,k}$ from the overlap-matrix error.
Defining the sampled-minus-exact overlap-block errors
\begin{equation}
\begin{aligned}
\Delta S_{cq}^{(\ell,s,k)}
=
S_{cq}^{\mathrm{samp},(\ell,s,k)} - S_{cq}^{\mathrm{exact},(\ell)},
\qquad
\Delta S_{qq}^{(\ell,s,k)}
=
S_{qq}^{\mathrm{samp},(\ell,s,k)} - S_{qq}^{\mathrm{exact},(\ell)},
\end{aligned}
\end{equation}
and a rank factorization
\begin{equation}
\Delta S_{cq}^{(\ell,s,k)} = Q^{(\ell,s,k)} R^{(\ell,s,k)},
\end{equation}
where $Q^{(\ell,s,k)}$ collects the independent classical directions that
appear in the sampled $cq$-block error, and $R^{(\ell,s,k)}$ records the
corresponding amplitudes of that error in those directions. In this
way, the factorization removes redundant information in
$\Delta S_{cq}^{(\ell,s,k)}$ before the threshold $\tau_{\ell,s,k}$ is
constructed; when the columns of $Q^{(\ell,s,k)}$ are orthonormal, one may
write $R^{(\ell,s,k)}=\left(Q^{(\ell,s,k)}\right)^\dagger
\Delta S_{cq}^{(\ell,s,k)}$,
we take
\begin{equation}
\begin{aligned}
D^{(\ell,s,k)} &=
\begin{bmatrix}
0 & R^{(\ell,s,k)} \\
\left(R^{(\ell,s,k)}\right)^\dagger &
\dfrac{\Delta S_{qq}^{(\ell,s,k)} + \Delta S_{qq}^{(\ell,s,k)\dagger}}{2}
\end{bmatrix}, \\
\tau_{\ell,s,k} &= \|D^{(\ell,s,k)}\|_2 .
\end{aligned}
\end{equation}

Let $\{v_{\ell,i}\}$ be the exact overlap-matrix modes for molecule $\ell$,
with eigenvalues $\sigma_{\ell,i}$, and let $c_0^{(\ell)}$ be the
corresponding exact ground-state vector. Expanding the ground state in
that basis,
\begin{equation}
\begin{aligned}
c_0^{(\ell)} = \sum_i a_{\ell,i} v_{\ell,i},
\qquad
w_{\ell,i} = |a_{\ell,i}|^2 .
\end{aligned}
\end{equation}
The unresolved weight for run $(\ell,s,k)$ is then defined by
\begin{equation}
W_{\mathrm{unres}}^{(\ell,s,k)}
=
\sum_{\sigma_{\ell,i} \le \tau_{\ell,s,k}} w_{\ell,i}.
\end{equation}
In words, $W_{\mathrm{unres}}^{(\ell,s,k)}$ is the total fraction of the
exact ground state that lies in overlap modes whose exact eigenvalue is
smaller than the sampled resolution threshold. The plotted quantity in
\cref{fig:appendix_plateau} is the seed average
\begin{equation}
W_{\mathrm{unres,mean}}(\ell,s)
=
\frac{1}{N_{\ell,s}}
\sum_{k=1}^{N_{\ell,s}} W_{\mathrm{unres}}^{(\ell,s,k)},
\end{equation}
where $N_{\ell,s}$ is the number of sampled runs for molecule $\ell$ at shot
count $s$.

As an empirical interpretation of the plateau behavior, molecules with
larger unresolved-overlap weight tend to show clearer plateau behavior
in panel (d) of \cref{fig:overlap_benchmark}. This
suggests that $W_{\mathrm{unres,mean}}(\ell,s)$ captures a relevant part of
the mechanism, and the underlying picture is physically plausible:
when a substantial fraction of the exact ground state lies in overlap
directions that are not resolved by the sampled matrices, improving the
overall sampling accuracy does not immediately translate into improved
energy convergence. At the same time, this quantity does not explain the
plateau quantitatively in all cases. For example, \ce{H4} already shows
relatively large unresolved weight at $10^5$ shots, whereas the plateau
in the sampled energy convergence becomes pronounced only at
$10^7$ shots. Therefore, although $W_{\mathrm{unres}}$ is the most
informative diagnostic we found, additional quantities will likely be
needed to explain the degree of the plateau more completely.

\begin{figure}[H]
\centering
\includegraphics[width=0.9\columnwidth]{figures/W_unres.png}
\caption{Seed-averaged unresolved-overlap weight
$W_{\mathrm{unres,mean}}(\ell,s)$ for each benchmark molecule at sampled
shot counts of $10^5$, $10^6$, and $10^7$.}
\label{fig:appendix_plateau}
\end{figure}

\clearpage
